# Supplementary material for: Breathing cluster in complex neuron-astrocyte networks
Source: arXiv:2302.00652 source file (2023-01-26)
Supplement: Supplementary file 1 [file Supplementary.pdf]

Supplementary Material for

# **Breathing cluster in complex neuron-astrocyte networks**

Ya Wang, Liang Wang, Huawei Fan, Jun Ma, Hui Cao, and Xingang Wang

Corresponding author: X. G. Wang (wangxg@snnu.edu.cn)

## **CONTENTS**

|                                                              |   |
|--------------------------------------------------------------|---|
| I. Coupling matrices of the original and simplified networks | 2 |
| II. Cluster breathing for parameter $a = 5 \times 10^{-2}$   | 2 |
| III. Coupling matrices of the larger-size neural network     | 3 |
| IV. Results for coupled Hodgkin-Huxley oscillators           | 4 |
| V. Results for noise-free system                             | 5 |

## I. COUPLING MATRICES OF THE ORIGINAL AND SIMPLIFIED NETWORKS

The adjacency matrix of the neural network plotted in Fig. 1(a) in the main text reads

$$A = \begin{pmatrix} 0 & 1 & 1 & 0 & 1 & 0 & 1 & 1 & 0 & 0 \\ 1 & 0 & 1 & 1 & 1 & 1 & 1 & 1 & 1 & 1 \\ 1 & 1 & 0 & 0 & 0 & 0 & 1 & 1 & 0 & 0 \\ 0 & 1 & 0 & 0 & 1 & 0 & 1 & 0 & 0 & 0 \\ 1 & 1 & 0 & 1 & 0 & 1 & 0 & 0 & 1 & 0 \\ 0 & 1 & 0 & 0 & 1 & 0 & 1 & 0 & 0 & 0 \\ 1 & 1 & 1 & 1 & 0 & 1 & 0 & 1 & 1 & 0 \\ 1 & 1 & 1 & 0 & 0 & 0 & 1 & 0 & 0 & 1 \\ 0 & 1 & 0 & 0 & 1 & 0 & 1 & 0 & 0 & 0 \\ 0 & 1 & 0 & 0 & 0 & 0 & 0 & 1 & 0 & 0 \end{pmatrix}, \quad (\text{S1.1})$$

The coupling matrix of the simplified network plotted in Fig. 4(a) in the main text reads

$$C = \begin{pmatrix} 0 & 1 & 1 & 0 & 1 & 0 & 1 & 1 \\ 1 & 0 & 1 & 3 & 1 & 1 & 1 & 1 \\ 1 & 1 & 0 & 0 & 0 & 0 & 1 & 1 \\ 0 & 1 & 0 & 0 & 1 & 0 & 1 & 0 \\ 1 & 1 & 0 & 3 & 0 & 0 & 0 & 0 \\ 0 & 1 & 0 & 0 & 0 & 0 & 0 & 1 \\ 1 & 1 & 1 & 3 & 0 & 0 & 0 & 1 \\ 1 & 1 & 1 & 0 & 0 & 1 & 1 & 0 \end{pmatrix}. \quad (\text{S1.2})$$

## II. CLUSTER BREATHING FOR PARAMETER $a = 5 \times 10^{-2}$

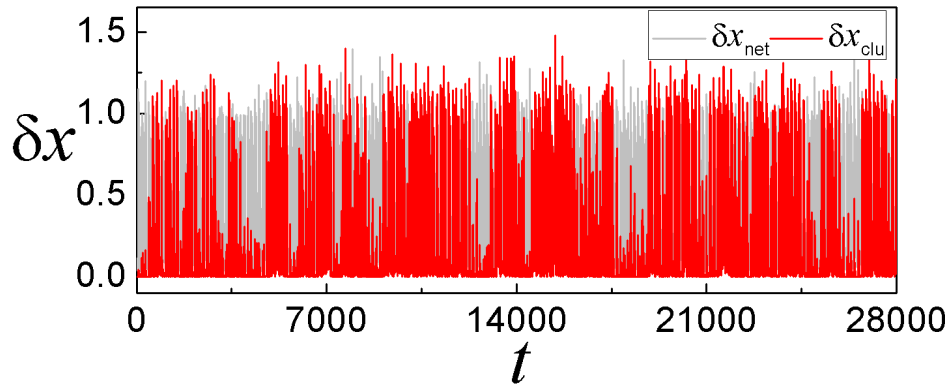

FIG. S1. *Cluster breathing for astrocyte parameter  $a = 5 \times 10^{-2}$ .* Shown is the time evolution of the network synchronization error,  $\delta x_{\text{net}}$  (grey color) and cluster synchronization error,  $\delta x_{\text{clu}}$  (red color). The other parameters are identical to Fig. 2 in the main text.

The breathing frequency of the cluster is dependent of the astrocyte parameters. In particular, with the increase of parameter  $a$ , the breathing frequency will be gradually increased, as depicted

in Fig. 3(a) in the main text. Shown in Fig. S1 is the time evolution of the network synchronization error,  $\delta x_{net}$  (grey color), and cluster synchronization error,  $\delta x_{clu}$  (red color), for parameter  $a = 5 \times 10^{-2}$ . Comparing with the result of  $a = 3 \times 10^{-2}$  (see Fig. 2 in the main text), the cluster is breathing at a higher frequency.

### III. COUPLING MATRICES OF THE LARGER-SIZE NEURAL NETWORK

For the neural network plotted in Fig. 5 in the main text ( $N = 20$ ), the adjacency matrix reads

$$A = \begin{pmatrix} 0 & 0 & 0 & 1 & 0 & 0 & 1 & 0 & 1 & 0 & 0 & 1 & 0 & 1 & 1 & 1 & 1 & 1 & 1 & 1 \\ 0 & 0 & 1 & 1 & 1 & 0 & 0 & 0 & 1 & 0 & 0 & 0 & 0 & 1 & 1 & 1 & 1 & 1 & 1 & 1 \\ 0 & 1 & 0 & 0 & 1 & 0 & 1 & 0 & 0 & 0 & 1 & 0 & 0 & 1 & 1 & 1 & 1 & 1 & 1 & 1 \\ 1 & 1 & 0 & 0 & 1 & 0 & 1 & 1 & 0 & 1 & 0 & 0 & 0 & 1 & 1 & 1 & 1 & 1 & 1 & 1 \\ 0 & 1 & 1 & 1 & 0 & 0 & 0 & 1 & 1 & 1 & 0 & 0 & 0 & 1 & 1 & 1 & 1 & 1 & 1 & 1 \\ 0 & 0 & 0 & 0 & 0 & 0 & 0 & 0 & 1 & 1 & 1 & 1 & 0 & 1 & 1 & 1 & 1 & 1 & 1 & 1 \\ 1 & 0 & 1 & 1 & 0 & 0 & 0 & 0 & 0 & 0 & 1 & 0 & 1 & 1 & 1 & 1 & 1 & 1 & 1 & 1 \\ 0 & 0 & 0 & 1 & 1 & 0 & 0 & 0 & 1 & 0 & 0 & 1 & 1 & 1 & 1 & 1 & 1 & 1 & 1 & 1 \\ 1 & 1 & 0 & 0 & 1 & 1 & 0 & 1 & 0 & 0 & 0 & 0 & 0 & 1 & 1 & 1 & 1 & 1 & 1 & 1 \\ 0 & 0 & 0 & 1 & 1 & 1 & 0 & 0 & 0 & 0 & 0 & 0 & 0 & 1 & 1 & 1 & 1 & 1 & 1 & 1 \\ 0 & 0 & 1 & 0 & 0 & 1 & 1 & 0 & 0 & 0 & 0 & 1 & 0 & 1 & 1 & 1 & 1 & 1 & 1 & 1 \\ 1 & 0 & 0 & 0 & 0 & 1 & 0 & 1 & 0 & 0 & 1 & 0 & 1 & 1 & 1 & 1 & 1 & 1 & 1 & 1 \\ 0 & 0 & 0 & 0 & 0 & 0 & 1 & 1 & 0 & 0 & 0 & 1 & 0 & 1 & 1 & 1 & 1 & 1 & 1 & 1 \\ 1 & 1 & 1 & 1 & 1 & 1 & 1 & 1 & 1 & 1 & 1 & 1 & 1 & 0 & 1 & 1 & 1 & 1 & 1 & 1 \\ 1 & 1 & 1 & 1 & 1 & 1 & 1 & 1 & 1 & 1 & 1 & 1 & 1 & 1 & 0 & 1 & 1 & 1 & 1 & 1 \\ 1 & 1 & 1 & 1 & 1 & 1 & 1 & 1 & 1 & 1 & 1 & 1 & 1 & 1 & 1 & 0 & 1 & 1 & 1 & 1 \\ 1 & 1 & 1 & 1 & 1 & 1 & 1 & 1 & 1 & 1 & 1 & 1 & 1 & 1 & 1 & 1 & 0 & 1 & 1 & 1 \\ 1 & 1 & 1 & 1 & 1 & 1 & 1 & 1 & 1 & 1 & 1 & 1 & 1 & 1 & 1 & 1 & 1 & 0 & 1 & 1 \\ 1 & 1 & 1 & 1 & 1 & 1 & 1 & 1 & 1 & 1 & 1 & 1 & 1 & 1 & 1 & 1 & 1 & 1 & 0 & 1 \\ 1 & 1 & 1 & 1 & 1 & 1 & 1 & 1 & 1 & 1 & 1 & 1 & 1 & 1 & 1 & 1 & 1 & 1 & 1 & 0 \end{pmatrix}, \quad (\text{S3.3})$$

and the coupling matrix of the simplified network ( $N' = 14$ ) reads

$$C = \begin{pmatrix} 0 & 0 & 0 & 1 & 0 & 0 & 1 & 0 & 1 & 0 & 0 & 1 & 0 & 7 \\ 0 & 0 & 1 & 1 & 1 & 0 & 0 & 0 & 1 & 0 & 0 & 0 & 0 & 7 \\ 0 & 1 & 0 & 0 & 1 & 0 & 1 & 0 & 0 & 0 & 1 & 0 & 0 & 7 \\ 1 & 1 & 0 & 0 & 1 & 0 & 1 & 1 & 0 & 1 & 0 & 0 & 0 & 7 \\ 0 & 1 & 1 & 1 & 0 & 0 & 0 & 1 & 1 & 1 & 0 & 0 & 0 & 7 \\ 0 & 0 & 0 & 0 & 0 & 0 & 0 & 0 & 1 & 1 & 1 & 1 & 0 & 7 \\ 1 & 0 & 1 & 1 & 0 & 0 & 0 & 0 & 0 & 0 & 1 & 0 & 1 & 7 \\ 0 & 0 & 0 & 1 & 1 & 0 & 0 & 0 & 1 & 0 & 0 & 1 & 1 & 7 \\ 1 & 1 & 0 & 0 & 1 & 1 & 0 & 1 & 0 & 0 & 0 & 0 & 0 & 7 \\ 0 & 0 & 0 & 1 & 1 & 1 & 0 & 0 & 0 & 0 & 0 & 0 & 0 & 7 \\ 0 & 0 & 1 & 0 & 0 & 1 & 1 & 0 & 0 & 0 & 0 & 1 & 0 & 7 \\ 1 & 0 & 0 & 0 & 0 & 1 & 0 & 1 & 0 & 0 & 1 & 0 & 1 & 7 \\ 0 & 0 & 0 & 0 & 0 & 0 & 1 & 1 & 0 & 0 & 0 & 1 & 0 & 7 \\ 1 & 1 & 1 & 1 & 1 & 1 & 1 & 1 & 1 & 1 & 1 & 1 & 1 & 0 \end{pmatrix}, \quad (\text{S3.4})$$

#### IV. RESULTS FOR COUPLED HODGKIN-HUXLEY OSCILLATORS

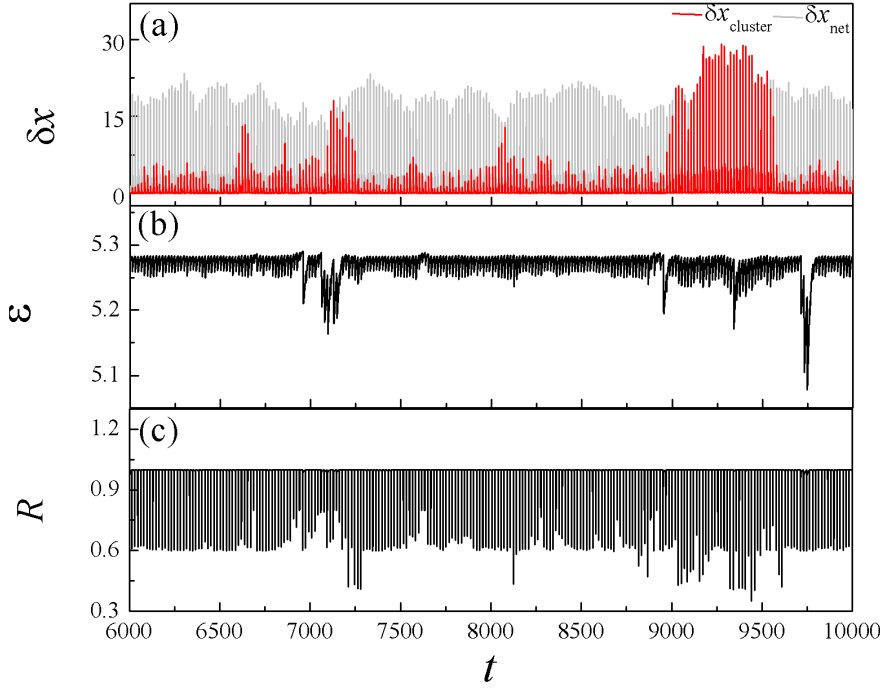

FIG. S2. *Breathing cluster in complex neuron-astrocyte network of coupled Hodgkin-Huxley(HH) oscillators.* (a) The time evolution of the network synchronization error,  $\delta x_{net}$  (grey color), and the cluster synchronization error,  $\delta x_{clu}$  (red color). (b) The time evolution of the uniform coupling strength,  $\epsilon(t)$ . (c) The time evolution of synchronization order parameter,  $R(t)$ .

The breathing phenomenon reported in the manuscript is also observed when adopting Hodgkin-Huxley (HH) oscillators as the neural dynamics. By the same network structure plotted in Fig. 1 in the main text, we describe the neural dynamics by HH oscillators and couple the oscillators by chemical synapses as described by Eq. (2) in the main text. The dynamics of the isolated HH oscillator is governed by equations

$$\begin{aligned} C_m \frac{dx}{dt} &= -\bar{g}_{Na} k_{Na} m^3 h (x - V_{Na}) - \bar{g}_K n^4 (x - V_K) - \bar{g}_L (x - V_L) + D\xi(t), \\ \frac{dy}{dt} &= \alpha_y(x)(1 - y) - \beta_y x, \text{ with } y = m, h, n. \end{aligned} \quad (\text{S4.5})$$

Here, we set the parameters as  $C_m = 1\text{F}/\text{cm}^2$ ,  $\bar{g}_{Na} = 120\text{mS}/\text{cm}^2$ ,  $\bar{g}_K = 36\text{mS}/\text{cm}^2$ ,  $\bar{g}_L = 0.3\text{mS}/\text{cm}^2$ ,  $V_{Na} = 50\text{mV}$ ,  $V_K = -77\text{mV}$ ,  $k_{Na} = 0.3$ , and  $V_L = 54.5\text{mV}$ . In Eq. (S4.5),  $\xi(t)$  represents noise perturbations, and the noise amplitude is set as  $D = 0.01$ . The opening rate  $\alpha_y$

and the closing rate  $\beta_y$ , ( $y = m, h, n$ ) are expressed as

$$\begin{aligned}
\alpha_m(x) &= \frac{0.1(x+40)}{1 - \exp[-(x+40)/10]}, \\
\beta_m(x) &= 4 \exp[-(x+65)/18], \\
\alpha_h(x) &= 0.07 \exp[-(x+65)/20], \\
\beta_h(x) &= \frac{1}{1 + \exp[-(x+35)/10]}, \\
\alpha_n(x) &= \frac{0.01(x+55)}{1 - \exp[-(x+55)/10]}, \\
\beta_n(x) &= 0.125 \exp[-(x+65)/80].
\end{aligned} \tag{S4.6}$$

As did for the HR oscillators in the main text, we couple the HH oscillators by excitatory chemical synapses, with the coupling current that neuron  $i$  receives from its neighbors being

$$I_c^i = \varepsilon(V_r - x_i) \sum_{j=1}^N a_{ij} h(x_j), \tag{S4.7}$$

where  $h(x_j) = [1 + e^{-\lambda(x_j - \alpha)}]^{-1}$  is the coupling function of chemical synapse and  $\varepsilon$  the coupling strength. Still, we set the coupling parameters as  $(V_r, \lambda, \alpha) = (2, 7.5, -0.25)$ .

Shown in Fig. S2(a) is the time evolution of the network synchronization error,  $\delta x_{net}$  (grey color), and the cluster synchronization error,  $\delta x_{clu}$  (red color). It is seen that the whole network is desynchronized throughout the process of system evolution, while the cluster is breathing slowly in a random fashion. The time evolution of the uniform coupling strength,  $\varepsilon(t)$ , and the synchronization order parameter,  $R(t)$ , are plotted in Figs. S2(b) and (c), respectively. It is seen that both  $\varepsilon(t)$  and  $R(t)$  are oscillating at a frequency much higher than that of cluster breathing.

## V. RESULTS FOR NOISE-FREE SYSTEM

Setting  $D = 0$  in Eq. (1) in the manuscript (noise-free neural oscillators) while keeping the other settings identical to Fig. 2 in the manuscript, we plot in Fig. S3 the time evolution of the network synchronization error,  $\delta x_{net}$  (grey color), and the cluster synchronization error,  $\delta x_{clu}$  (red color). It is seen that, similar to the results of noise-perturbed oscillators (see Fig. 2 in the main text), the cluster is still breathing intermittently at a frequency much slower than that of network desynchronization.

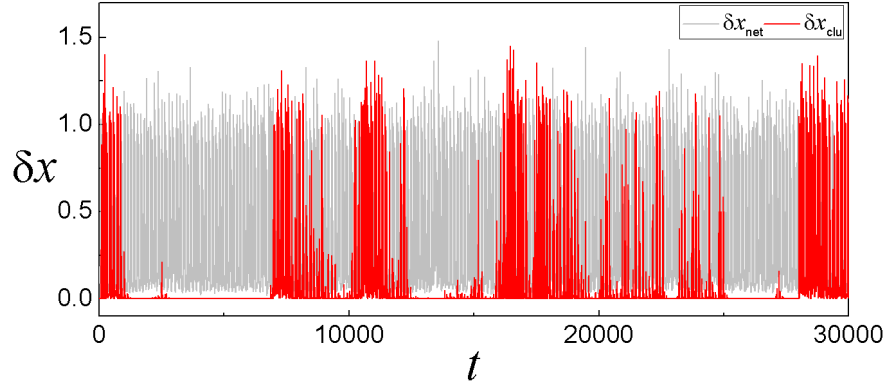

FIG. S3. *Cluster breathing in noise-free system.* For the same network model adopted in Fig. 2 in the main text but without noise perturbations, the time evolution of the network synchronization error,  $\delta x_{\text{net}}$  (grey color), and the cluster synchronization error,  $\delta x_{\text{clu}}$  (red color).
